# Supplementary material for: ERASER: A Benchmark to Evaluate Rationalized NLP Models
Source: arXiv:1911.03429 source file (2020-04-24)
Supplement: Supplementary file 1 [file acl2020_supplemental.tex]

%% this file exists for submission only; for camera ready the appendix should be in the main body of the paper.

\documentclass[11pt,a4paper]{article}
\usepackage{authblk}
\usepackage[hyperref]{acl2020}
\usepackage{times}
\usepackage{latexsym}
\usepackage{bbding}
\usepackage{pifont}
\usepackage{verbatim}
\usepackage{booktabs}
\usepackage{amsmath,amssymb,stmaryrd}  
\usepackage{MnSymbol}
\usepackage{graphicx}

\usepackage{url}

\usepackage[splitrule]{footmisc}
\interfootnotelinepenalty=10000
\usepackage[compact]{titlesec}
\usepackage{microtype}

\usepackage{bibentry}

\begin{document}
\input{sections/appendix.tex}

\nobibliography{acl2020}
\bibliographystyle{acl_natbib}
\end{document}
